# Supplementary material for: An end-to-end data-driven optimisation framework for constrained trajectories
Source: arXiv:2011.11820 source file (2021-02-05)
Supplement: Supplementary file 1 [file appendix.tex]

\subsection{Misc.}

\begin{proposition} \label{prop:phi_unitary}
    Let $\| \cdot \|_{\R^K}$ denote the Euclidean norm on $\R^K$ and let $\big\{ \lambda^{(d)} \big\}_{d=1}^D$ be a set of positive real numbers. Define the matrices $\Lambda \in \R^{D \times D}$ and $\overline{\Lambda} \in \R^{K \times K}$ as
    \begin{equation*}
        \Lambda := \left(
        \begin{array}{ccc}
                \lambda^{(1)} & & \\
                 & \ddots & \\
                 & & \lambda^{(D)}
            \end{array} \right) \qquad , \qquad
        \overline{\Lambda} := \left(
            \begin{array}{ccc}
                \lambda^{(1)} \, I_{K_1 + 1} & & \\
                 & \ddots & \\
                 & & \lambda^{(D)} I_{K_D + 1}
            \end{array} \right)
    \end{equation*}
    where $I_n$ is the identity matrix of size $n$. Then the operator $\Phi|_{\mathcal{Y}_\mathcal{K}} : \mathcal{Y}_\mathcal{K} \longrightarrow \R^K$ is bijective and satisfies
    \begin{equation*}
        \forall \, y \in \mathcal{Y}_\mathcal{K} \qquad \int_0^T \Big\| \Lambda^{\frac{1}{2}} \, y(t) \Big\|_{\R^D}^2 \, dt = \Big\| \overline{\Lambda}^\frac{1}{2} \, \Phi|_{\mathcal{Y}_\mathcal{K}} y \Big\|_{\R^K}^2 \; .
    \end{equation*}
\end{proposition}
\begin{proof}
    Let $y \in \mathcal{Y}_\mathcal{K}$ and let $c := \Phi|_{\mathcal{Y}_\mathcal{K}} y \in \R^{K_d}$. We have by the definition of the matrix $\Lambda$ and by the hypothesis $y \in \mathcal{Y}_\mathcal{K}$,
    \begin{equation*}
        \int_0^T \Big\| \Lambda^{\frac{1}{2}} \, y(t) \Big\|_{\R^D}^2 \, dt = \sum_{d=1}^D \lambda^{(d)} \int_0^T \Big| y^{(d)}(t) \Big|^2 \, dt = \sum_{d=1}^D \lambda^{(d)} \int_0^T \left| \sum_{k=0}^{K_d} c_k^{(d)} \, \varphi_k(t) \right|^2 dt \; ,
    \end{equation*}
    and the orthonormal property of the basis $\{\varphi_k\}_{k=0}^{+\infty}$ gives for all $d \in \{1,\dots,D\}$,
    \begin{equation*}
        \int_0^T \left| \sum_{k=0}^{K_d} c_k^{(d)} \, \varphi_k(t) \right|^2 dt = \sum_{k=0}^{K_d} \Big| c_k^{(d)} \Big|^2 \int_0^T \big| \varphi_k(t) \big|^2 \, dt = \sum_{k=0}^{K_d} \Big| c_k^{(d)} \Big|^2 \; .
    \end{equation*}
    By using the definition of $\overline{\Lambda}$, we obtain
    \begin{equation*}
        \int_0^T \Big\| \Lambda^{\frac{1}{2}} \, y(t) \Big\|_{\R^D}^2 \, dt = \sum_{d=1}^D \lambda^{(d)} \sum_{k=0}^{K_d} \Big| c_k^{(d)} \Big|^2 = \Big\| \overline{\Lambda}^\frac{1}{2} \, c \Big\|_{\R^K}^2 \; .
    \end{equation*}
    As a direct consequence, the operator $\Phi|_{\mathcal{Y}_\mathcal{K}} : \mathcal{Y}_\mathcal{K} \longrightarrow \R^K$ is injective. It is surjective as well since for all $\widetilde{c} = \big( \widetilde{c}_0^{(1)}, \dots, \widetilde{c}_{K_1}^{(1)}, \dots, \; \widetilde{c}_0^{(D)}, \dots, \widetilde{c}_{K_D}^{(D)} \big) \in \R^K$, the trajectory $\widetilde{y} \in \mathcal{Y}_\mathcal{K}$ defined by
    \begin{equation*}
        \forall \, d \in \{1,\dots,D\} \qquad \widetilde{y}^{(d)} := \sum_{k=0}^{K_d} \widetilde{c}_k^{(d)} \, \varphi_k
    \end{equation*}
    satisfies $\Phi|_{\mathcal{Y}_\mathcal{K}} \widetilde{y} = \Phi \widetilde{y} = \widetilde{c}$.
\end{proof}

\begin{definition}[Total fuel consumption]
    Let $\FF: \R^D \longrightarrow \R_+$ denote the fuel flow. We define the total fuel consumption $\TFC(y) \in \R_+$ of a trajectory $y \in L^2\big([0,T], \R^D\big)$ as follows:
    \begin{equation*}
        \TFC(y) := \int_0^T \FF\big(y(t) \big) \, dt \; .
    \end{equation*}
\end{definition}

\begin{definition} \label{def:phi}
    We define the integer $K := \sum_{d = 1}^D K_d$ and the operator $\Phi : L^2\big([0,T], \R^D \big) \longrightarrow \R^K$ as follows:
    \begin{equation*}
        \Phi y := \Big( c_1^{(1)}, \dots, c_{K_1}^{(1)}, \; c_1^{(2)}, \dots, c_{K_2}^{(2)}, \dots, \; c_1^{(D)}, \dots, c_{K_D}^{(D)} \Big) \; .
    \end{equation*}
\end{definition}

\begin{definition}
    We define
    \begin{enumerate}
        \item the projection operator $\Phi : \mathcal{C}\big([0,T], \R^D \big) \longrightarrow \R^K$ as follows:
        \begin{equation*}
            \Phi y := \Big( c_1^{(1)}, \dots, c_{K_1}^{(1)}, \; c_1^{(2)}, \dots, c_{K_2}^{(2)}, \dots, \; c_1^{(D)}, \dots, c_{K_D}^{(D)} \Big)^T \; ;
        \end{equation*}
        \item the set $\widetilde{\mathcal{D}}(y_0, y_T) \subset \R^K$ as the set of vectors satisfying the following linear condition:
        \begin{equation} \label{eq:endpoint_syst}
            A(0,T) \, c = \Gamma \; ,
        \end{equation}
        where the vector $\Gamma \in \R^{2D}$ is defined as
        \begin{equation*}
            \Gamma := \Big( y_0^{\ T} \quad y_T^{\ T} \Big)^T \; ,
        \end{equation*}
        and the matrix $A(0,T) \in \R^{2D \times K}$ is defined as
        \begin{equation*}
            A(0, T) := \left(
            \begin{array}{ccccccc}
                \varphi_1(0) & \dots & \varphi_{K_1}(0) & & & & \\
                & & & \ddots & & & \\
                & & & & \varphi_1(0) & \dots & \varphi_{K_D}(0) \\
                \varphi_1(T) & \dots & \varphi_{K_1}(T) & & & & \\
                & & & \ddots & & & \\
                & & & & \varphi_1(T) & \dots & \varphi_{K_D}(T) \\
            \end{array} \right) \; .
        \end{equation*}
    \end{enumerate}
\end{definition}

\begin{proposition} \label{prop:linear_const}
    \begin{enumerate}
        \item The restriction of the operator $\Phi$ to the subspace $\mathcal{Y}_\mathcal{K}$, namely $\Phi|_{\mathcal{Y}_\mathcal{K}} : \mathcal{Y}_\mathcal{K} \longrightarrow \R^K$, is bijective.
        \item A trajectory $y \in \mathcal{Y}_{\mathcal{K}}$ belongs to $\mathcal{D}(y_0, y_T)$ if and only if $\Phi y$ belongs to $\widetilde{\mathcal{D}}(y_0, y_T)$.
    \end{enumerate}
\end{proposition}
\begin{proof}
    \begin{enumerate}
        \item It is clear that each component $y^{(d)}$ of a trajectory $y \in \mathcal{Y}_\mathcal{K}$ is associated with a unique vector $c^{(d)} \in \R^{K_d}$ given by
        \begin{equation*}
            \forall \, k = 1, \dots, K_d \qquad c_k^{(d)} = \int_0^T y^{(d)}(t) \, \varphi_{k}(t) \, dt \; .
        \end{equation*}
        Since the restriction $\Phi|_{\mathcal{Y}_\mathcal{K}}$ is actually the Cartesian product of the bijective functions $\Phi^{(d)} : \text{span} \left\{ \varphi_{k} \right\}_{k = 1}^{K_d} \longrightarrow \R^{K_d}$ defined by
        \begin{equation*}
            \Phi^{(d)} y^{(d)} := c^{(d)} \; ,
        \end{equation*}
        it inherits the bijective nature of its components. This proves the first point.
        \item Let $y \in \mathcal{Y}_\mathcal{K}$ and let $c := \Phi y \in \R^K$. By the definition of the matrix $A(0,T)$, we have
        \begin{align*}
            A(0,T) c
                & = A(0,T) \Big( c_1^{(1)}, \dots, c_{K_1}^{(1)}, \; c_1^{(2)}, \dots, c_{K_2}^{(2)}, \dots, \; c_1^{(D)}, \dots, c_{K_D}^{(D)} \Big)^T \\
                & = \left( \sum_{k=1}^{K_1} c_k^{(1)} \varphi_k(0), \dots, \displaystyle \sum_{k=1}^{K_D} c_k^{(D)} \varphi_k(0), \dots, \sum_{k=1}^{K_1} c_k^{(1)} \varphi_k(T), \dots, \sum_{k=1}^{K_D} c_k^{(D)} \varphi_k(T) \right)^T \\
                & = \big( y(0) \quad y(T) \big)^T \; .
        \end{align*}
        The conclusion follows directly from the preceding relation.
    \end{enumerate}
\end{proof}

\begin{remark}
    Throughout the paper, we will use interchangeably the two following representations of a vector $c \in \R^K$:
    \begin{itemize}
        \item $c = (c_1, c_2, \dots, c_K)^T$;
        \item $c = \Big( c_1^{(1)}, \dots, c_{K_1}^{(1)}, \; c_1^{(2)}, \dots, c_{K_2}^{(2)}, \dots, \; c_1^{(D)}, \dots, c_{K_D}^{(D)} \Big)^T$.
    \end{itemize}
    Indeed, for any $k \in \{1, \dots, K\}$, there exists a unique\footnote{Appendix ?} $\big(\widetilde{d}, \widetilde{k}\big)$ such that
    \begin{equation*}
        k = \widetilde{k} + \sum_{d = 1}^{\widetilde{d}-1} K_d \; ,
    \end{equation*}
    with $\widetilde{d} \in \{1,\dots,D\}$ and $\widetilde{k} \in \{1, \dots, K_{\widetilde{d}} \}$. In this case, we have $c_k = c_{\widetilde{k}}^{(\widetilde{d})}$.
\end{remark}

\subsection{Interpretation}

\begin{proposition} \label{prop:min_pb_equiv_y_C}
    A vector $c^\star \in \R^K$ is solution of the optimisation problem \eqref{eq:opt_c} if and only if the trajectory $y^\star := \Phi|_{\mathcal{Y}_\mathcal{K}}^{-1} c^\star \in \mathcal{Y}_\mathcal{K}$ is solution of the following optimisation problem
    \begin{equation*}
        y^\star \in \argmin_{y \in \mathcal{Y}_\mathcal{K} \cap \mathcal{B}(y_0, y_T)} \sum_{i=1}^I \omega_i \int_0^T \Big\| \Lambda^{\frac{1}{2}} \big( y(t) - y_{R_i}(t) \big) \Big\|_{\R^D}^2 \, dt + \int_0^T \FF\big(y(t) \big) \, dt \; .
    \end{equation*}
\end{proposition}
\begin{proof}
     First of all, we define the maps $g_1: \R^K \longrightarrow \R$ as
    \begin{equation*}
        g_1(c) := \sum_{i=1}^I \omega_i \, \Big\| \overline{\Lambda}^{\frac{1}{2}} \big(c - c_{R_i} \big) \Big\|_{\R^K}^2 + \TFC\big( \Phi|_{\mathcal{Y}_\mathcal{K}}^{-1} c \big) \; ,
    \end{equation*}
    and $g_2: L^2\big([0,T], \R^d \big) \longrightarrow \R$ as
    \begin{equation*}
        g_2(y) := \sum_{i=1}^I \omega_i \int_0^T \Big\| \Lambda^{\frac{1}{2}} \big( y(t) - y_{R_i}(t) \big) \Big\|_{\R^D}^2 \, dt + \int_0^T \FF\big(y(t) \big) \, dt \; .
    \end{equation*}
    Let $c \in \R^K$ and let $y := \Phi|_{\mathcal{Y}_\mathcal{K}}^{-1} c \in \mathcal{Y}_\mathcal{K}$ be its associated trajectory. By the definition of $y$, we clearly have
    \begin{equation*}
        \TFC\big( \Phi|_{\mathcal{Y}_\mathcal{K}}^{-1} c \big) = \TFC(y) = \int_0^T \FF\big(y(t) \big) \, dt \; .
    \end{equation*}
    Furthermore Proposition \ref{prop:phi_unitary} implies
    \begin{equation*}
        \sum_{i=1}^I \omega_i \, \Big\| \overline{\Lambda}^{\frac{1}{2}} \big(c - c_{R_i} \big) \Big\|_{\R^K}^2 = \sum_{i=1}^I \omega_i \int_0^T \Big\| \Lambda^{\frac{1}{2}} \Big( y(t) - y_{R_i}(t) \Big) \Big\|_{\R^D}^2 \, dt \; ,
    \end{equation*}
    showing that $g_1(c) = g_2\big(y\big)$. Since the set $\mathcal{C}(y_0, y_T)$ is the image of $\mathcal{Y}_\mathcal{K} \cap \mathcal{B}(y_0, y_T)$ under the bijection $\Phi|_{\mathcal{Y}_\mathcal{K}}$ by definition, it follows that minimising the map $g_1$ over the set $\mathcal{C}(y_0, y_T)$ amounts to minimising the function $g_2$ over $\mathcal{Y}_\mathcal{K} \cap \mathcal{B}(y_0, y_T)$.
\end{proof}

\subsection{Quadratic cost for a convex optimisation problem} \label{subsec:quad_model}

\todo{Note ? + Change the position of $\kappa$ and adapt the results}\\
We focus on the case where the function $f$ (defining the cost $F$) is quadratic. In this setting, explicit formulas for the objective functions appearing in the optimisation problems \eqref{eq:opt_proj} and \eqref{eq:opt_proj_2} can be established. In particular this permits to derive sufficient conditions on the parameter $\kappa > 0$ so that the optimisation problems are proved to be equivalent to quadratic programs \citep[Sec. 4.4]{convexopt}, namely the objective functions are convex quadratic. In practice, this allows to make use of efficient convex optimisation libraries to solve numerically the problems.

Throughout this subsection, we suppose that the function $f$ defining the cost $F$ is quadratic, \emph{i.e.}
\begin{equation} \label{eq:quad_f}
    f(x) = x^T Q x + w^T x + r = \sum_{d_1, d_2 = 1}^D Q_{d_1 d_2} \, x^{(d_1)} \, x^{(d_2)} +  \sum_{d = 1}^D w_d \, x^{(d)} + r \; ,
\end{equation}
where $x \in \R^D$, $Q \in \R^{D \times D}$ is symmetric, $w \in \R^D$ and $r \in \R$. We define now some vectors and matrices which will be used to prove the quadratic programming property.

\begin{definition} \label{def:misc}
    We define
    \begin{enumerate}
        \item the map $\widetilde{\varphi} \in \mathcal{C}\big([0,T], \R^K\big)$ as
        \begin{equation*}
            \widetilde{\varphi} := \Big( \varphi_1, \dots, \varphi_{K_1}, \; \varphi_1, \; \dots, \varphi_{K_2}, \dots, \; \varphi_1, \dots, \varphi_{K_D} \Big)^T \; ;
        \end{equation*}
        \item the matrix $\widetilde{Q} \in \R^{K \times K}$ as
        \begin{equation*}
            \widetilde{Q} := \left(
            \begin{array}{ccc}
                Q_{11} \, J_{K_1, K_1} & \ldots & Q_{1D} \, J_{K_1, K_D} \\
                \vdots & & \vdots \\
                Q_{D1} \, J_{K_D, K_1} & \ldots & Q_{DD} \, J_{K_D, K_D}
            \end{array} \right) \; ,
        \end{equation*}
        where $J_{n,m}$ is the all-ones matrix of size $n \times m$;
        \item the matrix $\overline{Q} \in \R^{K \times K}$ as
        \begin{equation*}
	        \overline{Q}_{k_1 k_2} :=  \widetilde{Q}_{k_1 k_2} \int_0^T \widetilde{\varphi}_{k_1}(t) \, \widetilde{\varphi}_{k_2}(t) \, dt \; ;
        \end{equation*}
        \item the matrix $\overline{Q}_V := V^T \overline{Q} V \in \R^{K \times K}$ which can be written as follows:
        \begin{equation*}
            \overline{Q}_V = \left( \begin{array}{cc}
                \overline{Q}_{V, 11} & \overline{Q}_{V, 12} \\[2mm]
                \overline{Q}_{V, 21} & \overline{Q}_{V, 22}
            \end{array} \right) \; ,
        \end{equation*}
        where $\overline{Q}_{V, 11} \in \R^{\sigma \times \sigma}$, $\overline{Q}_{V, 12} \in \R^{\sigma \times (K - \sigma)}$, $\overline{Q}_{V, 21} \in \R^{(K-\sigma) \times \sigma}$ and $\overline{Q}_{V, 22} \in \R^{(K-\sigma) \times (K-\sigma)}$;
        \item the vector $\widetilde{w} \in \R^K$ as
        \begin{equation*}
            \widetilde{w} := \big( w_1 \, J_{1, K_1} \quad \dots \quad w_D \, J_{1, K_D} \big)^T \; ;
        \end{equation*}
        \item the vector $\overline{w} \in \R^K$ as
        \begin{equation*}
	        \overline{w}_k := \widetilde{w}_k \int_0^T \widetilde{\varphi}_k(t) \, dt \; ;
        \end{equation*}
        \item the vector $\overline{w}_V := V^T \overline{w} \in \R^K$ which can be written as follows:
        \begin{equation*}
            \overline{w}_V = \Big( \overline{w}_{V, 1}^{\ T} \quad \overline{w}_{V, 2}^{\ T} \Big)^T
        \end{equation*}
        where $\overline{w}_{V, 1} \in \R^\sigma$ and $\overline{w}_{V, 2} \in \R^{K-\sigma}$.
    \end{enumerate}
\end{definition}

\begin{remark}
    The matrix $\widetilde{Q}$ inherits the symmetric property of $Q$. Indeed, since $J_{n, m}^{\ T} = J_{m, n}$ and $Q_{d_1 d_2} = Q_{d_2 d_1}$, we have
    \begin{equation*}
        \widetilde{Q}^T = \left(
        \begin{array}{ccc}
            Q_{11} \, J_{K_1, K_1}^{\ T} & \ldots & Q_{D1} \, J_{K_D, K_1}^{\ T} \\
            \vdots & & \vdots \\
            Q_{1D} \, J_{K_1, K_D}^{\ T} & \ldots & Q_{DD} \, J_{K_D, K_D}^{\ T}
        \end{array} \right) = \left(
        \begin{array}{ccc}
            Q_{11} \, J_{K_1, K_1} & \ldots & Q_{1D} \, J_{K_1, K_D} \\
            \vdots & & \vdots \\
            Q_{D1} \, J_{K_1, K_D} & \ldots & Q_{DD} \, J_{K_D, K_D}
        \end{array} \right) = \widetilde{Q} \; .
    \end{equation*}
    It follows that the matrices $\overline{Q}$ and $\overline{Q}_V$ are also symmetric.
\end{remark}

The following lemma provides quadratic formulas for the costs $\check{F}: \R^K \longrightarrow \R$ and $\widetilde{F}: \R^\sigma \longrightarrow \R$ in the present setting. They will be used to establish sufficient conditions so that the optimisation problems are convex. 

\begin{lemma} \label{lem:ff}
    Suppose that the function $f$ is of the form \eqref{eq:quad_f}. Then
    \begin{enumerate}
        \item we have for all $c \in \R^K$,
        \begin{equation*}
            \check{F}(c) = c^T \overline{Q} c + \overline{w}^T c + r T \; ;
        \end{equation*}
        \item we have for all $\widetilde{c}_1 \in \R^\sigma$,
        \begin{equation*}
            \widetilde{F}(\widetilde{c}_1) = \widetilde{c}_1^T \, \overline{Q}_{V, 11} \, \widetilde{c}_1 + \Big( 2 \, \overline{Q}_{V, 12} \, \widetilde{c}_{2,3} + \overline{w}_{V, 1}^{\ T} \Big)^T \widetilde{c}_1 + \widetilde{c}_{2,3}^{\ T} \, \overline{Q}_{V, 22} \, \widetilde{c}_{2,3} + \overline{w}_{V, 2}^{\ T} \, \widetilde{c}_{2,3} + r T \; ,
        \end{equation*}
        where $\widetilde{c}_{2,3} := \Big( c_{R_i}^{\ T} V_2 \quad \Gamma^T U \big(S_{A,2}^{-1}\big)^T \Big)^T \in \R^{K - \sigma}$ and $i$ is arbitrarily chosen in $\{1, \dots, I \}$.
    \end{enumerate}
\end{lemma}
\begin{proof}
    Let $c \in \R^K$ and let $y := \Phi|_{\mathcal{Y}_\mathcal{K}}^{-1} c \in \mathcal{Y}_\mathcal{K}$ be its associated trajectory, which can be represented as follows:
    \begin{equation*}
        \forall \, d \in \{1, \dots, D\} \qquad y^{(d)} = \sum_{k=1}^{K_d} c_k^{(d)} \, \varphi_k \; .
    \end{equation*}
    We also remark that each component of the vector
    \begin{equation*}
        c = \Big( c_1^{(1)}, \dots, c_{K_1}^{(1)}, \; c_1^{(2)}, \dots, c_{K_2}^{(2)}, \dots, \; c_1^{(D)}, \dots, c_{K_D}^{(D)} \Big)^T
    \end{equation*}
    can be simply described by a single parameter so that we can write $c = (c_1, c_2, \dots, c_K)^T$.
    \begin{enumerate}
        \item By inserting the preceding representation of $y$ into \eqref{eq:quad_f}, we obtain:
        \begin{align*}
    	    f\big( y(t) \big)
    		    & = \sum_{d_1, d_2 = 1}^D \sum_{k_1 = 0}^{K_{d_1}} \sum_{k_2 = 0}^{K_{d_2}} Q_{d_1 d_2} \, c_{k_1}^{(d_1)} c_{k_2}^{(d_2)} \, \varphi_{k_1}(t) \varphi_{k_2}(t) + \sum_{d = 1}^D \sum_{k=0}^{K_d} w_d \, c_k^{(d)} \, \varphi_k(t) + r \; ,
        \end{align*}
        for all $t \in [0,T]$. The next step of the proof consists in changing the indices of the vectors and matrices. Using the above rewriting of $c$ as well as the matrix $\widetilde{Q}$ and the map $\widetilde{\varphi}$ given in \cref{def:misc} provides the following equality:
        \begin{equation*}
            \sum_{d_1, d_2 = 1}^D \sum_{k_1 = 0}^{K_{d_1}} \sum_{k_2 = 0}^{K_{d_2}} Q_{d_1 d_2} \, c_{k_1}^{(d_1)} c_{k_2}^{(d_2)} \, \varphi_{k_1}(t) \varphi_{k_2}(t) = \sum_{k_1, k_2 = 1}^{K} \widetilde{Q}_{k_1 k_2} \, c_{k_1} \, c_{k_2} \, \widetilde{\varphi}_{k_1}(t) \widetilde{\varphi}_{k_2}(t) \; .
        \end{equation*}
        By similar computations, we obtain
        \begin{equation*}
            \sum_{d = 1}^D \sum_{k=0}^{K_d} w_d \, c_k^{(d)} \, \varphi_k^{(d)}(t) = \sum_{k = 1}^{K} \widetilde{w}_k \, c_k \, \widetilde{\varphi}_k(t) \; ,
        \end{equation*}
        leading to
        \begin{align*}
    	    f\big(y(t) \big) = \sum_{k_1, k_2 = 1}^{K} \widetilde{Q}_{k_1 k_2} \, c_{k_1} \, c_{k_2} \, \widetilde{\varphi}_{k_1}(t) \widetilde{\varphi}_{k_2}(t) + \sum_{k = 1}^{K} \widetilde{w}_k \, c_k \, \widetilde{\varphi}_k(t) + r \; .
        \end{align*}
        Integrating finally over $[0,T]$ gives
        \begin{align*}
            \check{F}(c)
                & = \int_0^T f\big(y(t)\big) \, dt \\
    		    & = \sum_{k_1, k_2 = 1}^{K} \widetilde{Q}_{k_1 k_2} \int_0^T \widetilde{\varphi}_{k_1}(t) \, \widetilde{\varphi}_{k_2}(t) \, dt \, c_{k_1} \, c_{k_2} + \sum_{k = 1}^{K} \widetilde{w}_k \int_0^T \widetilde{\varphi}_k(t) \, dt \, c_k + r T \\
    		    & = \sum_{k_1, k_2 = 1}^{K} \overline{Q}_{k_1 k_2} \, c_{k_1} \, c_{k_2} + \sum_{k = 1}^{K} \overline{w}_k \, c_k + r T \\
    		    & = c^T \overline{Q} c + \overline{w}^T c + r T \; .
        \end{align*}
        \item By the definition of $\widetilde{F}$ given in \cref{subsec:modelling}, we have
        \begin{equation*}
            \widetilde{F}(\widetilde{c}_1) = \check{F}\Big( V \big( \widetilde{c}_1^T \quad \widetilde{c}_{2,3}^{\ T} \big)^T \Big) \; .
        \end{equation*}
        We use now the result of the preceding point and the definitions of the matrix $\overline{Q}_V$ and the vector $\overline{w}_V$ to obtain
        \begin{align*}
            \widetilde{F}(\widetilde{c}_1)
                & = \big( \widetilde{c}_1^T \quad \widetilde{c}_{2,3}^{\ T} \big) \big( V^T \overline{Q} V \big) \big( \widetilde{c}_1^T \quad \widetilde{c}_{2,3}^{\ T} \big)^T + \big( V^T \overline{w} \big)^T \big( \widetilde{c}_1^T \quad \widetilde{c}_{2,3}^{\ T} \big)^T + r T \\
                & = \big( \widetilde{c}_1^T \quad \widetilde{c}_{2,3}^{\ T} \big) \overline{Q}_V \big( \widetilde{c}_1^T \quad \widetilde{c}_{2,3}^{\ T} \big)^T + \overline{w}_V^T \big( \widetilde{c}_1^T \quad \widetilde{c}_{2,3}^{\ T} \big)^T + r T \\
                & = \widetilde{c}_1^T \, \overline{Q}_{V, 11} \, \widetilde{c}_1 + \widetilde{c}_1^T \, \overline{Q}_{V, 12} \, \widetilde{c}_{2,3} + \widetilde{c}_{2,3}^{\ T} \, \overline{Q}_{V, 21} \, \widetilde{c}_1 + \widetilde{c}_{2,3}^{\ T} \, \overline{Q}_{V, 22} \, \widetilde{c}_{2,3} \\
                & \hspace{1cm} + \overline{w}_{V, 1}^{\ T} \, \widetilde{c}_{1} + \overline{w}_{V, 2}^{\ T} \, \widetilde{c}_{2,3} + r T \; .
        \end{align*}
        Rearranging the preceding terms and using the fact that $\overline{Q}_V$ is symmetric gives the result.
    \end{enumerate}
\end{proof}

\todo{Changer la place de $\kappa$ dans fonction coût ?}\\
In the present setting, the optimisation problem \eqref{eq:opt_proj} is then equivalent to the following quadratic one:
\begin{equation} \label{eq:opt_proj_quad}
    \left\{
    \begin{array}{l}
         \displaystyle \widetilde{c}_1^\star \in \argmin_{\widetilde{c}_1 \in \R^\sigma} \sum_{i=1}^I \omega_i \, \big( \widetilde{c}_1 - \widetilde{c}_{R_i, 1} \big)^T \Lambda_{\Sigma,1}^{-1} \big( \widetilde{c}_1 - \widetilde{c}_{R_i, 1} \big) \\
         \hspace{2cm} + \kappa \, \Big( \widetilde{c}_1^T \, \overline{Q}_{V, 11} \, \widetilde{c}_1 + \Big( 2 \, \overline{Q}_{V, 12} \, \widetilde{c}_{2,3} + \overline{w}_{V, 1}^{\ T} \Big)^T \widetilde{c}_1 \Big) \\[2mm]
         \widetilde{c}_2 = V_2^T c_{R_i} \\[2mm]
         \widetilde{c}_3 = S_{A,2}^{-1} \, U^T \Gamma
    \end{array} \; .
    \right.
\end{equation}
In the following result, we provide sufficient conditions on the parameter $\kappa > 0$ so that the problem \eqref{eq:opt_proj_quad} is a quadratic program. The proof uses the fact that the symmetric matrix associated with the quadratic objective function is now explicit and given by the sum of two matrices. A perturbation result for matrices is then applied to obtain a bound for $\kappa$ assuring that the symmetric matrix is positive semidefinite.

\begin{theorem} \label{thm:quad_prog}
    Let $\rho_1 \geqslant \rho_2 \geqslant \dots \geqslant \rho_\sigma$ and $\lambda_1 \geqslant \lambda_2 \geqslant \dots \geqslant \lambda_K$ be respectively the eigenvalues of the symmetric matrices $\overline{Q}_{V, 11}$ and $\Sigma$.
    \begin{enumerate}
        \item If $\rho_\sigma \geqslant 0$ then the optimisation problem \eqref{eq:opt_proj_quad} is a quadratic program for any $\kappa > 0$.
        \item If $\rho_\sigma < 0$ then the optimisation problem \eqref{eq:opt_proj_quad} is a quadratic program for any $\kappa > 0$ satisfying
        \begin{equation*}
            \kappa < - \frac{1}{\lambda_1 \, \rho_\sigma} \; .
        \end{equation*}
    \end{enumerate}
\end{theorem}
\begin{proof}
    We first note that all the eigenvalues of the matrix $\Sigma$ are non-negative (because $\Sigma$ is a covariance matrix) and that $\lambda_{\sigma + 1} = \dots = \lambda_K = 0$ (because $\rk \Sigma = \sigma$). In particular, the eigenvalue $\lambda_1$ is positive.\\
    Standard calculations show that the symmetric matrix associated with the quadratic objective function of the problem \eqref{eq:opt_proj_quad} is given by
    \begin{equation*}
        M(\kappa) := \kappa \, \overline{Q}_{V, 11} + \Lambda_{\Sigma, 1}^{-1} \in \R^{\sigma \times \sigma} \; .
    \end{equation*}
    Let $\mu_1(\kappa) \geqslant \mu_2(\kappa) \geqslant \dots \geqslant \mu_\sigma(\kappa)$ denote the eigenvalues of $M(\kappa)$. Our goal is to prove that $\mu_\sigma(\kappa)$ is non-negative to assure that $M$ is positive semidefinite. Since $M(\kappa)$ can be interpreted as a perturbed version of $\Lambda_{\Sigma, 1}^{-1}$, we can apply Weyl's inequality (see for instance \citet{wang201965}) which implies
    \begin{equation*}
        \kappa \, \rho_\sigma + \frac{1}{\lambda_1} \leqslant \mu_\sigma(\kappa) \; .
    \end{equation*}
    We distinguish now the two cases.
    \begin{enumerate}
        \item In the case where $\rho_\sigma \geqslant 0$ (\emph{i.e.} the matrix $\overline{Q}_{V, 11}$ is positive semidefinite), then $\mu_\sigma(\kappa)$ is positive for any $\kappa > 0$.
        \item If $\rho_\sigma < 0$ and $\kappa \leqslant - \frac{1}{\lambda_1 \, \rho_\sigma}$ then $\mu_\sigma(\kappa)$ is non-negative.
    \end{enumerate}
\end{proof}

For the sake of completeness, we finish by rewriting the problem \eqref{eq:opt_proj_quad} as a quadratic optimisation problem in $\mathcal{V}_1 \subset \R^K$ with affine constraints function.

\begin{proposition} \label{prop:quad_min_pb}
    Suppose that the function $f$ is of the form \eqref{eq:quad_f}. Then the optimisation problem \eqref{eq:opt_proj_quad} is equivalent to the following one:
    \begin{equation} \label{eq:quad_min_pb}
        c^\star \in \argmin_{c \in \mathcal{V}_1} c^T \Big( \kappa \, \overline{Q} + \Sigma^\dagger \Big) c + \left( \kappa \, \overline{w} - 2 \sum_{i=1}^I \omega_i \, \Sigma^\dagger c_{R_i} \right)^{\hspace{-5pt}T} c \; .
    \end{equation}
\end{proposition}
\begin{proof}
    As explained above and according to \cref{prop:opt_equiv}, the problem \eqref{eq:opt_proj_quad} is equivalent to the problem \eqref{eq:opt_proj_2} in the present setting. Hence it is sufficient to show that the objective functions $g_1, g_2: \R^K \longrightarrow \R$ defined as
    \begin{itemize}
        \item $\displaystyle g_1(c) := \sum_{i=1}^I \omega_i \, \big( c - c_{R_i} \big)^T \Sigma^\dagger \big( c - c_{R_i} \big) + \kappa \, \check{F}(c)$ ,
        \item $\displaystyle g_2(c) := c^T \Big( \kappa \,  \overline{Q} + \Sigma^\dagger \Big) c + \left( \kappa \, \overline{w} - 2 \sum_{i=1}^I \omega_i \, \Sigma^\dagger c_{R_i} \right)^{\hspace{-5pt}T} c$ .
    \end{itemize}
    have the same minima. Firstly we have by standard calculations,
    \begin{align*}
        \sum_{i=1}^I \omega_i \, \big( c - c_{R_i} \big)^T \Sigma^\dagger \big( c - c_{R_i} \big)
        & = \sum_{i=1}^I \omega_i \, c^T \Sigma^\dagger c - 2 \sum_{i=1}^I \omega_i \, c_{R_i}^{\ T} \Sigma^\dagger c + \sum_{i=1}^I \omega_i \, c_{R_i}^{\ T} \Sigma^\dagger c_{R_i} \\
        & = c^T \Sigma^\dagger c - \left( 2 \sum_{i=1}^I \omega_i \, \Sigma^\dagger  c_{R_i} \right)^{\hspace{-5pt}T} c + \sum_{i=1}^I \omega_i \, c_{R_i}^{\ T} \Sigma^\dagger c_{R_i} \; ,
    \end{align*}
    for any $c \in \R^K$, where we have used $\sum_{i=1}^I \omega_i = 1$. Combining now this equality with \cref{lem:ff} implies
    \begin{align*}
        g_1(c)
            & = c^T \Sigma^\dagger c - \left( 2 \sum_{i=1}^I \omega_i \, \Sigma^\dagger  c_{R_i} \right)^{\hspace{-5pt}T} c + \sum_{i=1}^I \omega_i \, c_{R_i}^{\ T} \Sigma^\dagger c_{R_i} + \kappa \, \Big( c^T \overline{Q} c + \overline{w}^T c + r T \Big) \\
            & = c^T \Big( \kappa \, \overline{Q} + \Sigma^\dagger \Big) c + \left( \kappa \, \overline{w} - 2 \sum_{i=1}^I \omega_i \, \Sigma^\dagger c_{R_i} \right)^{\hspace{-5pt}T} c + \sum_{i=1}^I \omega_i \, c_{R_i}^{\ T} \Sigma^\dagger c_{R_i} + \kappa \, r T \\
            & = g_2(c) + \sum_{i=1}^I \omega_i \, c_{R_i}^{\ T} \Sigma^\dagger c_{R_i} + \kappa \, r T \; .
    \end{align*}
    Since the two last terms of the last right-hand side do not depend on $c$, we deduce that the objective functions $g_1$ and $g_2$ have the same minima.
\end{proof}
